# Supplementary material for: Strengthening Deterministic Policies for POMDPs
Source: arXiv:2007.08351 source file (2020-07-16)
Supplement: Supplementary file 1 [file 08-appendix.tex]

\appendix

\section{Proof of Theorem~\ref{th_state}}

We want to prove that state splitting yields a bisimilar POMDP. To do so we first
introduce bisimulations~\cite{GivanDG03}, adapting the standard notion from MDPs
to POMDPs in the straightforward way.

\begin{definition}[Bisimulation]
    Let $\pomdp = (\mdp, \obss, \obs)$ be a POMDP with underlying MDP
    $\mdp=(S,\sinit,\acts,\prob)$, a reward function $\rew$, and
    a labeling function $L:S\to 2^{AP}$ that assigns to each state a
    set of atomic propositions from a finite set $AP$.

    A \emph{bisimulation}
    on $\pomdp$ is an equivalence relation ${\approx}\subseteq S\times S$
    such that for all $s,s'\in S$ with $s\approx s'$ we have
    \begin{enumerate}
        \item $\lambda(s)=\lambda(s')$ and $L(s) = L(s')$,
        \item for all $\act\in\acts(s)$ and all equivalence classes $C\in S/{\approx}$:
            \[
            \sum_{t\in C}\prob(s,\act,t) = \sum_{t'\in C}\prob(s',\act,t')
            \]
        \item $\rew(s,\act) = \rew(s',\act)$ for all $\act\in\acts(s)$.
    \end{enumerate}
    Two states $s,s'$ are called \emph{bisimilar} if there is a bisimulation $\approx$ with
    $s\approx s'$.
\end{definition}

The labeling function $L$ introduced here for POMDPs is used, e.\,g., in temporal logics,
to refer to sets of states with certain properties. For reachability properties, all
target states can be assigned a ``target'' label.

This definition of bisimilarity can be extended for relating states of different POMDPs:
Let $\pomdp$ and $\pomdp'$ be two POMDPs.
We call them bisimilar ($M\approx M'$) if there is a bisimulation on the disjoint union of
their state spaces that relates the initial states of the two POMDPs.

It is well known that bisimilar states satisfy (among others) the same CTL and LTL properties,
including reachability, discounted reward, and steady-state properties.

\begin{theorem}
    Let $\pomdp = (\mdp,\obss,\obs)$ be a POMDP with $\mdp=(S,\sinit,\acts,\prob)$,
    reward function $\rew$ and labeling function $L$.
    Let $\pomdp' = (\mdp',\obss,\obs')$ with $\mdp'=(S',\sinit,\acts,\prob')$,
    reward function $\rew'$ and labeling function $L'$ result from $\pomdp$ by splitting state $s\in S$, i.\,e.,
    \begin{itemize}
        \item $\states' := \bigl(\states\setminus\{s\}\bigr)\dcup\bigl\{ (s,z,\alpha)\,\big|\,(z,\alpha)\in\text{pred}_\pomdp(s)\bigr\}$,
        \item for all $t\in\states'$:
            \begin{align*}
                \obs'(t) &:= \begin{cases}
                    \obs(s) & \text{if $t = (s, z,\alpha)$ for some $z\in\obss$ and $\alpha\in\acts$,} \\
                    \obs(t) & \text{otherwise;}
                \end{cases} \\
                L'(t) &:= \begin{cases}
                    L(s) & \text{if $t = (s, z,\alpha)$ for some $z\in\obss$ and $\alpha\in\acts$,} \\
                    L(t) & \text{otherwise;}
                \end{cases}
            \end{align*}
        \item for all $t,t'\in\states'$, $\beta\in\acts$:
            \[
            \prob'(t,\beta,t') = \begin{cases}
                    \prob(t,\beta,t') & \text{if $t,t'\in\states\setminus\{s\}$,} \\
                    \prob(s,\beta,s)  & \text{if $t=(s,z,\alpha)$ and $t' = (s,z,\beta)$} \\
                                      & \text{\qquad for some $z\in\obss$ and $\alpha\in\acts$,} \\
                    \prob(t,\beta,s)  & \text{if $t\in\states\setminus\{s\}$ and $t'=(s,\obs(t),\beta)$,} \\
                    \prob(s,\beta,t') & \text{if $t=(s,z,\alpha)$ for some $z\in\obss$} \\
                                      & \text{\qquad and $\act\in\acts$ and $t'\in\states\setminus\{s\}$,}\\
                    0                 & \text{otherwise;}
                \end{cases}
            \]
        \item for all $t\in\states'$ and $\beta\in\acts(t)$:
            \[
                \rew'(t,\beta) := \begin{cases}
                    \rew(s,\beta) & \text{if $t = (s, z,\act)$ for some $z\in\obss$ and $\act\in\acts$,} \\
                    \rew(t,\beta) & \text{otherwise.}
                \end{cases}
            \]
    \end{itemize}
    Then $\pomdp$ and $\pomdp'$ are bisimilar.
\end{theorem}

\begin{proof}
    We denote the states of $\pomdp$ with $s,t,\ldots$ and the corresponding
    states of $\pomdp'$ by $s',t',\ldots$
    We construct an equivalence relation on $S\dcup S'$ as follows:
    \[
        {\approx} := \bigl\{ t, t'\,\big|\,t\in S\setminus\{s\}\bigr\}^2
            \dcup
            \bigl\{s, (s,z,\act)\,\big|\, (z,\act)\in \text{pred}_\pomdp(s) \bigr\}^2
    \]
    It is easy to see that $\approx$ is a bisimulation with $\sinit\approx\sinit'$, i.\,e., $\pomdp$ and $\pomdp'$
    are bisimilar.\qed
\end{proof}
